# Supplementary material for: SGD on Neural Networks Learns Functions of Increasing Complexity
Source: arXiv:1905.11604 source file (2019-05-28)
Supplement: Supplementary file 1 [file extra_plots_etc_from_appendix.tex]

\begin{figure*}[h!]
\begin{center}
\begin{tabular} {cccc}
  \includegraphics[width=1.2in]{./distribution_bad} &
  \includegraphics[width=1.2in]{./linear_bad} &
  \includegraphics[width=1.2in]{./sgd_bad} &
  \includegraphics[width=1.2in]{./info_lin_bad} \\
  \includegraphics[width=1.2in]{./distribution_good} &
  \includegraphics[width=1.2in]{./linear_good} &
  \includegraphics[width=1.2in]{./sgd_good} &
  \includegraphics[width=1.2in]{./info_lin_good} \\
  \end{tabular}
\end{center}
  \caption{A distribution admitting several good linear classifiers. The data are 
    A higher-complexity model trained with SGD will often yield linear decision boundary even in the late stages of training. However, conditioning on the wrong}
  \label{fig:many_linear}
\end{figure*}

Notice (about the train-test plot):
\begin{enumerate}[(i)]
    \item The number of SGD steps is often thought of as a proxy for the ``complexity'' of the model (or implicitly, a proxy for ``number of parameters''). There are several plausible justifications for this \cite{} \pnote{norm bounds, SGD-stability}).
    \item Classically, we expect the gap between train and set to grow with increasing complexity of the classifiers.
    However, we do not observe this gap increasing unboundedly as SGD training progresses. \pnote{We already discussed this a bit above... sounds repetitive. Also, make a plot for the what we classically expect?}
\end{enumerate}
It is particularly striking that such ``extreme overfitting'' -- fitting the train set exactly --  somehow does not
destroy the test error.

\pnote{move this "overparameterized" notion somewhere else..}

\dnote{Talk concretely about UC bounds and high Rademacher complexity as the two reasons why classical theory doesn't explain generalization in NNs? We somehow blend it here}

traditionally you get a training set and you don't have to know anything about the test set. and this is how you generalize. We don't attempt to come up with criteria like that. We are trying to explain. 

Moreover, even in the cases where the ERM that we find is good in terms of generalization, it is observed that the test error saturates and does not improve with training defying the claim that train and test performance have to be close as illustrated in Fig~\ref{fig1}.

The only explanation for the generalization performance of neural networks
is that the choice of optimization algorithm is important: In practice, we do not find an arbitrary Empirical Risk Minimizer (ERM), but rather, we find an ERM by running Stochastic Gradient Descent (SGD) or its variants from a randomly-initialized network.
%There must therefore be something special about the minima which SGD finds, which leads it towards networks that generalize.
The natural question that arises is:
% This motivates our current work.
% We are interested in answering:
\begin{center}
\textit{How do the dynamics of SGD on neural networks, under real-world input distributions, lead to minima that generalize well?}
\end{center}

\begin{figure}
    \centering
    \begin{subfigure}{0.6\textwidth}
            \centering
            \includegraphics[width=\textwidth]{./table_intro_small.png}
            \caption{Behavior of conditional mutual information}
    \end{subfigure}%
    \begin{subfigure}{0.3\textwidth}
            \centering
            \includegraphics[width=.8\textwidth]{./CIfar10_ana_info.png}
            \caption{Step 10}
    \end{subfigure}%
    \caption{SGD training on a 3-layer, 100-width dense neural network.
    Data distribution is an isotropic Gaussian in 2-dimensions, labeled by a linear classifier with 10\% label noise. The blue line corresponds to the decision boundary of the neural network which becomes more ``linear'' before starting overfitting to the label noise.}
    \label{fig:gaussian2dim}
\end{figure}

\begin{figure*}[!ht]
\begin{center}

\begin{tabular} {cc}
 \includegraphics[width=2in, clip]{./noisy_norm_info.png}

 \includegraphics[width=2in, clip]{./CIfar10_ana_info.png}
 
\end{tabular}

\caption{Mutual information of the best linear classifier and CNN on the task of classifying CIFAR10 images to two categories, Animals and Objects.} 
\label{fig1} 

\end{center}
\end{figure*}

\section{Related Work}

Allen-Zhu continuation:
\emph{
\begin{itemize}
    \item They do not characterize the "shape" of the function being learned -- it may do as well as the linear model, but not because it is ``essentially linear''
    in our sense.
    (it's possible the proof techniques work though).
    \item Their results are quantitatively weak: If the data distribution is linearly-separable  (plus small label noise)
    with margin $\gamma$, an application of their Theorem says we can learn it with $exp(\gamma)$ samples, and size of network. (TODO, check this).
    In contrast, we claim our results even with $0$-margin (eg: gaussian data w/ linear separator).
    \item We show the "linear learning" more generally, for deeper networks.
\end{itemize}}

    \begin{figure*}[!htb]
\begin{center}
\includegraphics[width=3in, clip]{./yy_zoom_out_info.png}
\end{center}
\caption{\bnote{Is this referenced anywhere?}}
\end{figure*}

\begin{figure*}[!htb]
\begin{center}
\begin{tabular} {cc}
  \includegraphics[width=1.7in, clip]{./Into_yy_distribution.png} & 
  \includegraphics[width=2in, clip]{./yy_info.png}\\
  \end{tabular}
  \begin{tabular} {cccc}
  \includegraphics[width=1.45in, clip]{./Intro_yy_random.png}
  \includegraphics[width=1.45in, clip]{./Intro_yy_one_epoch.png}
  \includegraphics[width=1.45in, clip]{./Intro_yy_100_epochs.png}
  \includegraphics[width=1.45in, clip]{./Intro_yy_1000_epochs.png}\\
  \end{tabular}
\end{center}
  \caption{Convergence of NNs on Yin-Yang distribution}
  \label{fig:ex2}
\end{figure*}

\begin{figure*}[!htb]
\begin{center}
\includegraphics[width=3in, clip]{./introfig1.png} 
\end{center}
\caption{A representative example of train and test loss curves.}
\label{fig5}
\end{figure*}

\begin{figure}[!htb]
    \centering
    \begin{subfigure}{0.25\textwidth}
            \centering
            \includegraphics[width=\textwidth]{./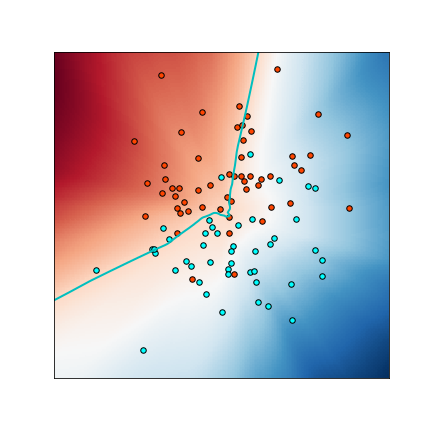}
            \caption{Initialization}
    \end{subfigure}%
    \begin{subfigure}{0.25\textwidth}
            \centering
            \includegraphics[width=\textwidth]{./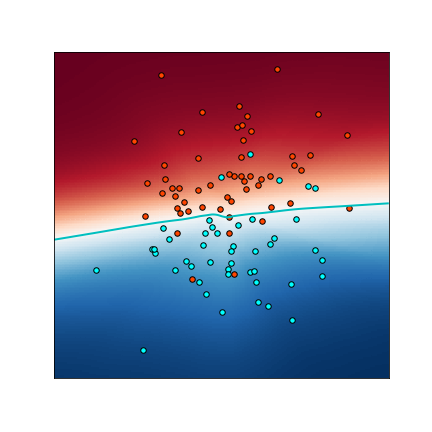}
            \caption{Simple concept}
    \end{subfigure}%\\
    \begin{subfigure}{0.25\textwidth}
            \centering
            \includegraphics[width=\textwidth]{./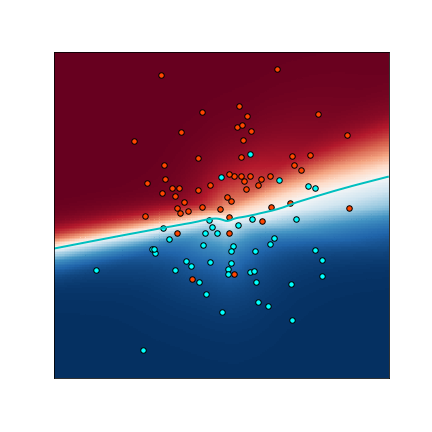}
            \caption{Complex concept}
    \end{subfigure}%
    \begin{subfigure}{0.25\textwidth}
            \centering
            \includegraphics[width=\textwidth]{./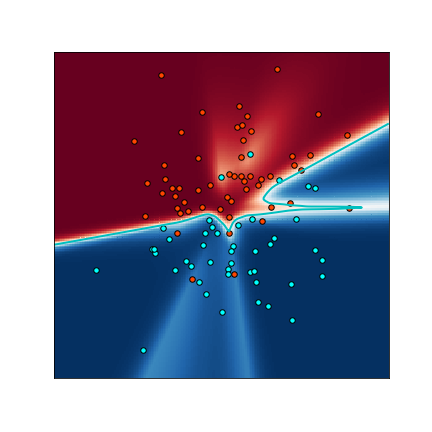}
            \caption{Overfit}
    \end{subfigure}
\end{figure}
